# Supplementary material for: Fractal fluctuations at mixed-order transitions in interdependent networks
Source: arXiv:2208.00440 source file (2022-07-31)
Supplement: Supplementary file 1 [file SI.pdf]

SUPPLEMENTARY MATERIAL

# Fractal fluctuations at mixed-order transitions in interdependent networks

Bnaya Gross,[1] Ivan Bonamassa,[1,2] and Shlomo Havlin[1]

[1]*Department of Physics, Bar Ilan University, Ramat Gan, Israel*

[2]*Department of Network and Data Science, CEU, Quellenstrasse 51, A-1100 Vienna, Austria*

(Dated: July 29, 2022)

## I. FLUCTUATIONS AWAY FROM CRITICALITY

In contrast to the character of critical fluctuations at the hybrid transition threshold, whose profile was found to best fit a skewed Gaussian distribution (see Fig. 2**b**, Fig. 3**b** in the main text and Fig. S3 in what below), the character of fluctuations away from criticality follows a classical Gaussian distribution (Fig. S1**a**). Away from the hybrid criticality, therefore, we expect a customary square-root scaling $\sigma(M) \sim \sqrt{N} = L^{d/2}$, as shown in Fig. S1**b**.

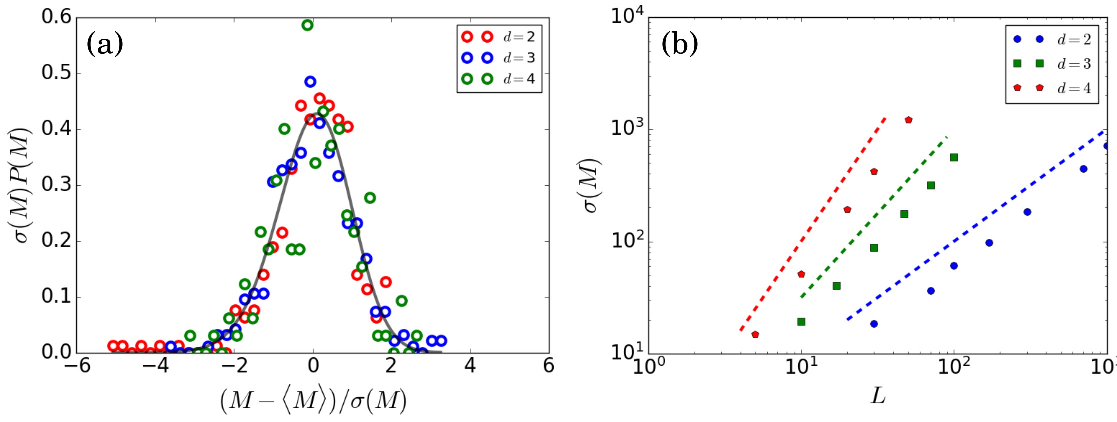


FIG. S1: **Fluctuations away from criticality. (a)** The fluctuations away from criticality ($\Delta p \gg 0$) are found to be Gaussian. Here we used $L = 30$. **(b)** The fluctuations follow the known scaling $\sigma(M) \sim \sqrt{N} = L^{d/2}$ (dashed lines). Simulations (markers) are shown for $\Delta p = 5 \cdot 10^{-2}$.

## II. INTERDEPENDENT MAGNETIZATION

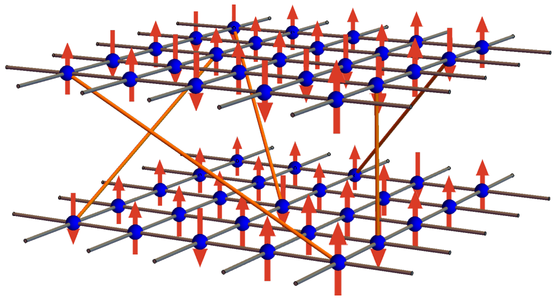

FIG. S2: **Pictorial representation of the randomly interdependent $2D$ Ising model.**

The interdependent Ising spins model was first introduced in Ref. [1]. The magnetic evolution of the networks is modeled using Glauber dynamics [2] as follow. In the uncoupled case, a randomly chosen spin $\sigma_i$ is flipped with probability $w(\sigma_i) = (1 + \exp\{2\beta\mathcal{J}k_i\sigma_i\Sigma_i\})^{-1}$ where $\beta = 1/T$, $k_i = \sum_j A_{ij}$ is the degree of node $i$ and $\Sigma_i \equiv \frac{1}{k_i}\sum_j A_{ij}\sigma_j$ is the effective field created at node $i$ by its neighbors. Once the networks are coupled and node $i$ becomes interdependent on node $i'$ in the other network (see Fig. S2), the flipping probability of node $i$, $w(\sigma_i)$, adaptively changes and depends on the magnetic state of $i'$, which can be approximated by its local magnetic field $\Sigma_{i'}$. Thus, the flipping probability of node $i$ in network $A$ which is thermally coupled to node $i'$ in network $B$ is updated to $w_i^{A\leftarrow B} = (1 + \exp\{2\beta\mathcal{J}k_i^A\sigma_i^A\Sigma_i^A\Sigma_{i'}^B\})^{-1}$. At each temperature, spins are chosen randomly and being flipped according to the interdependent flipping probability until the system reaches an equilibrium and the total magnetization is measured. As described in the main text, the model undergoes a spontaneous hybrid first-order magnetization transition at a finite critical temperature for any dimension $d \geq 2$ of the underlying lattices.

## III. PDFS OF THE INTERDEPENDENT MAGNETIZATION MODEL

The distributions $P(T_c)$ and $P(M_c)$ of the interdependent spins model are shown in Fig. S3 and they are found to best fit skewed Gaussian as reported in Eq.(5) in the main text (see also the caption of Fig.3 for more details). The shapes of the distributions are similar to those found for interdependent percolation (see Fig. 2**b** and Fig. 3**b** in the main text) despite the differences between the two models.

## IV. FRACTAL FLUCTUATIONS IN INTERDEPENDENT RANDOM NETWORKS

In the main text we presented the fractal fluctuation phenomenon in randomly interdependent $d$-dimensional lattices. We confirm here that this critical phenomenon occurs also in randomly interdependent random networks. In Fig. S4 we show both for interdependent percolation and

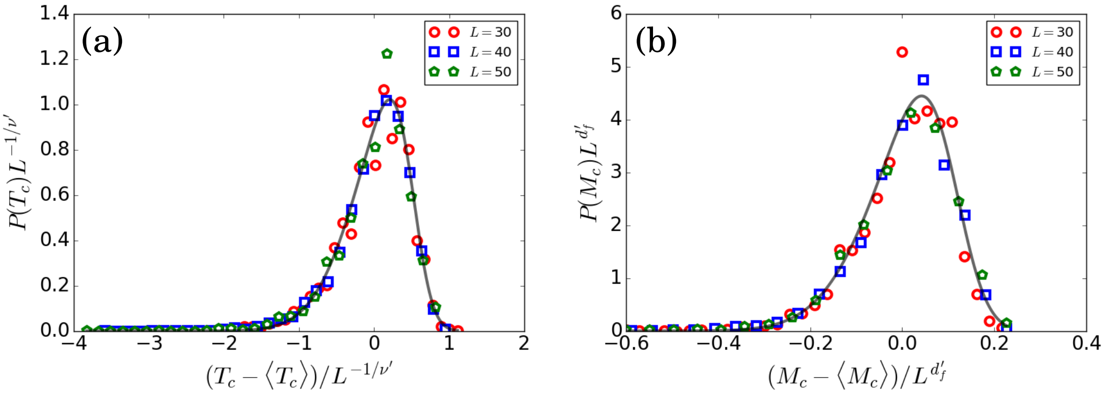


FIG. S3: **Fluctuations distributions at hybrid transitions in interdependent spins lattices.** (**a**) The distribution of critical temperatures, $P(T_c)$, for different $L$ collapses according to an equation analogous to Eq. (5) in the main text, where now $p_c$ is replaced by $T_c$. The distribution is a skewed Gaussian with $\gamma_1 \simeq -0.683$ and $\kappa = 0.526$. (**b**) The distribution of the critical magnetization, $P(M_c)$, for different $L$ collapses according to an equation analogous to the one for $P(M_c)$ reported in the caption to Fig.3 in the main text. Again, the distribution is a skewed Gaussian with $\gamma_1 \simeq -0.574$ and $\kappa = 0.418$. Simulations are shown for $d = 2$.

interdependent magnetization on Erdős-Rényi networks that the fluctuations are non-fractal away from the mixed-order critical threshold, they crossover to a critical fractal behavior close to criticality below the correlation length. Since the fractal dimension is $d'_f = 3d/4$ and the scaling in Eq. (3) in the main text is defined in terms of the linear size of the lattices, $L$, we here advance a general scaling relation for random graphs in terms of their system's size, $N$, given by:

$$\sigma(M_c) \sim N^{3/4}. \tag{S1}$$

At long scales, i.e. above the correlation length $\xi'$, the fluctuations are not-critical and follow a Gaussian scaling form

$$\sigma(M) \sim N^{1/2}. \tag{S2}$$

Fig. S4 displays the crossover from Eq. (S1) at small values of $N$ to Eq. (S2) at large values of $N$. The crossover point depends on the displacement from criticality $\Delta p$ ($\Delta T$).

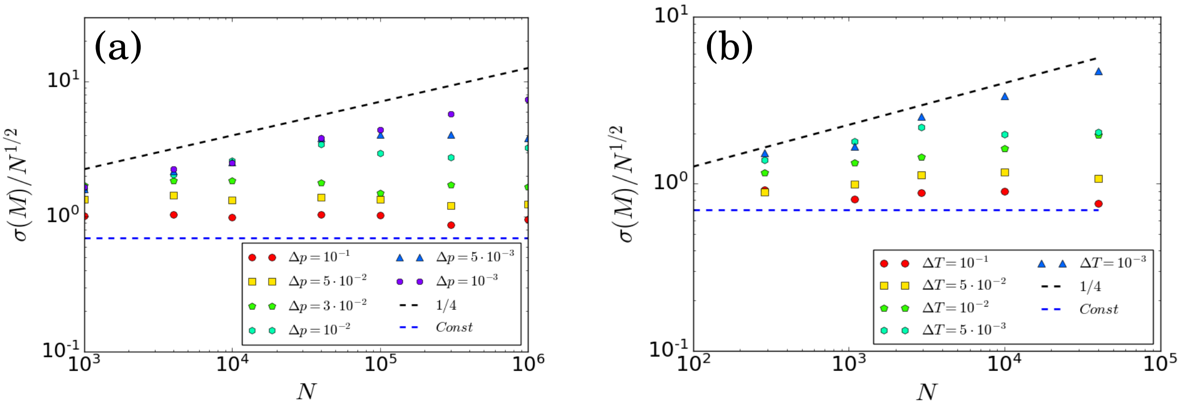


FIG. S4: **Fractal fluctuations in interdependent ER networks.** The fractal fluctuations phenomenon appears also at the mixed-order percolation transition in interdependent random network for both **(a)** percolation and **(b)** magnetization processes. For small values of $N$ (below the correlation length $\xi'$) the scaling follow Eq. (S1) while for large values of $N$ (above the correlation length) the scaling follows Eq. (S2). The crossover between the two behaviours depends on $\Delta p$ ($\Delta T$).

| $d$ | $L$ | $m$ | $L$ | $m$ | $L$ | $m$ | $L$ | $m$ | $L$ | $m$ | $L$ | $m$ |
|---|---|---|---|---|---|---|---|---|---|---|---|---|
| 2 | 10 | 400 | 30 | 400 | 70 | 400 | 100 | 400 | 300 | 400 | 1000 | 400 |
| 3 | 8 | 215 | 10 | 350 | 15 | 88 | 30 | 371 | 70 | 182 | 100 | 52 |
| 4 | 5 | 400 | 8 | 400 | 10 | 400 | 14 | 56 | 20 | 400 | 30 | 118 |
| 5 | 5 | 400 | 8 | 400 | 10 | 400 | 14 | 175 | 20 | 17 | - | - |
| 6 | 3 | 400 | 4 | 350 | 5 | 400 | 6 | 362 | 8 | 400 | 10 | 172 |
| 7 | 3 | 400 | 4 | 191 | 5 | 400 | 6 | 145 | 8 | 105 | 10 | 27 |

TABLE I: **Statistics of samples : interdependent percolation.** List of the samples' sizes gathered to analyze the statistics of the percolation thresholds $p_c$ and of the critical mass of the MGCC, $M_c$, for the mixed-order percolation phase transitions in randomly interdependent $d$-dimensional lattices.

| $d$ | $L$ | $m$ | $L$ | $m$ | $L$ | $m$ | $L$ | $m$ | $L$ | $m$ |
|---|---|---|---|---|---|---|---|---|---|---|
| 2 | 10 | 500 | 30 | 75 | 50 | 42 | 70 | 89 | 100 | 22 |
| 3 | 5 | 100 | 7 | 100 | 10 | 100 | 20 | 48 | 30 | 60 |
| 4 | 4 | 100 | 6 | 100 | 8 | 75 | 12 | 32 | 14 | 26 |
| 5 | 3 | 100 | 4 | 100 | 5 | 73 | 6 | 107 | 9 | 174 |
| 6 | 3 | 100 | 4 | 100 | 5 | 46 | 6 | 35 | 7 | 16 |
| 7 | 2 | 159 | 3 | 131 | 4 | 61 | 5 | 88 | 6 | 25 |

TABLE II: **Statistics of samples : interdependent magnetization.** Samples' sizes for the analysis of the ferromagnetic-to-paramagnetic thresholds, $T_c$, and the magnetization critical mass, $M_c$, for the mixed-order magnetization transition in randomly interdependent $d$-dimensional Ising-spin lattices.


[1] Ivan Bonamassa, Bnaya Gross, and Shlomo Havlin. Interdependent couplings map to thermal, higher-order interactions. *arXiv preprint arXiv:2110.08907*, 2021.

[2] Pavel L Krapivsky, Sidney Redner, and Eli Ben-Naim. *A kinetic view of statistical physics*. Cambridge University Press, 2010.
